# Supplementary material for: Accurate and efficient localized basis sets for two-dimensional materials
Source: arXiv:2411.12566 source file (2024-11-22)
Supplement: Supplementary file 1 [file SM.pdf]

# SUPPLEMENTARY MATERIAL
# Accurate and efficient localized basis sets for two-dimensional materials

Daniel Bennett,[1,*] Michele Pizzochero,[2,1,†] Javier Junquera,[3] and Efthimios Kaxiras[1,4]

[1]*John A. Paulson School of Engineering and Applied Sciences, Harvard University, Cambridge, Massachusetts 02138, USA*
[2]*Department of Physics, University of Bath, Bath BA2 7AY, United Kingdom*
[3]*Departamento de Ciencias de la Tierra y Física de la Materia Condensada, Universidad de Cantabria, Avenida de los Castros, s/n, E-39005 Santander, Spain*
[4]*Department of Physics, Harvard University, Cambridge, Massachusetts 02138, USA*

## CONTENTS

Optimized Basis Sets 2
Graphene 2
SZP 2
SZPF 2
DZP 2
DZPF 3
TZP 3
TZPF 3
QZP 3
QZPF 4
hBN 4
SZP 4
SZPF 5
DZP 5
DZPF 6
TZP 6
TZPF 7
QZP 7
QZPF 8

Native Basis Sets 8
Graphene 8
SZP 8
SZPF 8
DZP 9
DZPF 9
TZP 9
TZPF 10
QZP 10
QZPF 10
hBN 10
SZP 10
SZPF 11
DZP 11
DZPF 12
TZP 12
TZPF 13

* dbennett@seas.harvard.edu
† mp2834@bath.ac.uk

QZP 13
QZPF 14

## OPTIMIZED BASIS SETS

### Graphene

*SZP*

```
%Block PAO.Basis
C    3      0.99941
 n=2   0   1   E   132.56520    4.52564
     6.00093
     1.00000
 n=2   1   1   E     6.06390    6.06460
     6.71080
     1.00000
 n=3   2   1   E    14.47828    4.32078
     6.22538
     1.00000
%EndBlock PAO.Basis
```

*SZPF*

```
%Block PAO.Basis
C    4      0.72944
 n=2   0   1   E    42.12421    4.75046
     6.82785
     1.00000
 n=2   1   1   E    68.63006    5.51880
     6.38924
     1.00000
 n=3   2   1   E     6.69187    2.05040
     6.61759
     1.00000
 n=4   3   1   E    12.14453    4.45904
     6.38671
     1.00000
%EndBlock PAO.Basis
```

*DZP*

```
%Block PAO.Basis
C    3      0.47301
 n=2   0   2   E   128.93712    5.06736
     6.06851     4.37818
     1.00000     1.00000
 n=2   1   2   E   125.09083    5.55843
     6.06164     4.10885
     1.00000     1.00000
 n=3   2   1   E   241.27541    0.31346
     5.51134
     1.00000
%EndBlock PAO.Basis
```

*DZPF*

```
%Block PAO.Basis
C    4      -0.19231
 n=2   0   2   E      8.64983       5.16910
     6.26642      4.43682
     1.00000      1.00000
 n=2   1   2   E    104.59443       4.19280
     6.38064      4.71071
     1.00000      1.00000
 n=3   2   1   E    163.55969       0.17394
     4.89617
     1.00000
 n=4   3   1   E     10.64167       3.30969
     6.70618
     1.00000
%EndBlock PAO.Basis
```

*TZP*

```
%Block PAO.Basis
C    3      -0.46133
 n=2   0   3   E      9.61267       3.95672
     6.44810      4.58129      2.69608
     1.00000      1.00000      1.00000
 n=2   1   3   E     15.32030       5.12231
     6.69902      4.56886      2.63727
     1.00000      1.00000      1.00000
 n=3   2   1   E    233.03757       0.06888
     5.15455
     1.00000
%EndBlock PAO.Basis
```

*TZPF*

```
%Block PAO.Basis
C    4      -0.27459
 n=2   0   3   E     53.57167       6.21003
     6.71585      4.67684      2.69082
     1.00000      1.00000      1.00000
 n=2   1   3   E    125.78914       5.68034
     6.70503      4.67099      2.67594
     1.00000      1.00000      1.00000
 n=3   2   1   E    246.27832       0.00714
     5.41225
     1.00000
 n=4   3   1   E     67.84555       0.39218
     5.81824
     1.00000
%EndBlock PAO.Basis
```

*QZP*

```
%Block PAO.Basis
C    3      -0.33496
```

```
  n=2   0   4   E    47.25003    5.76808
     6.45715    4.62636    2.50283    1.53287
     1.00000    1.00000    1.00000    1.00000
  n=2   1   4   E   102.44223    5.72268
     6.53473    4.71879    2.95343    2.15789
     1.00000    1.00000    1.00000    1.00000
  n=3   2   1   E   203.45534    0.13083
     5.19147
     1.00000
%EndBlock PAO.Basis
```

*QZPF*

```
%Block PAO.Basis
C    4     -0.31777
  n=2   0   4   E    69.96820    4.04549
     6.00502    4.24411    2.65622    2.22922
     1.00000    1.00000    1.00000    1.00000
  n=2   1   4   E    99.13869    6.04351
     6.87035    4.93582    2.83332    2.07361
     1.00000    1.00000    1.00000    1.00000
  n=3   2   1   E   235.49474    0.02652
     5.46558
     1.00000
  n=4   3   1   E    90.15417    1.31836
     5.50057
     1.00000
%EndBlock PAO.Basis
```

**hBN**

*SZP*

```
%Block PAO.Basis
B    3      0.95338
  n=2   0   1   E   102.31261    3.35267
     6.74023
     1.00000
  n=2   1   1   E     5.19112    3.71284
     6.50022
     1.00000
  n=3   2   1   E     5.19423    1.33172
     6.43542
     1.00000
N    3      0.40811
  n=2   0   1   E    79.28779    5.48281
     6.00467
     1.00000
  n=2   1   1   E   133.08018    0.62142
     6.46868
     1.00000
  n=3   2   1   E     5.28432    4.19460
     6.39965
     1.00000
%EndBlock PAO.Basis
```

*SZPF*

```
%Block PAO.Basis
B      4         0.97838
  n=2     0     1     E      51.30016        6.41709
        6.92700
        1.00000
  n=2     1     1     E      92.24670        5.83911
        6.44009
        1.00000
  n=3     2     1     E      10.28435        0.00995
        6.29224
        1.00000
  n=4     3     1     E       5.07643        2.37707
        6.31242
        1.00000
N      4         0.59572
  n=2     0     1     E     211.09560        4.90352
        6.18382
        1.00000
  n=2     1     1     E      16.92610        5.66821
        6.27281
        1.00000
  n=3     2     1     E      66.28899        3.57328
        5.84485
        1.00000
  n=4     3     1     E       8.25259        2.27276
        6.30817
        1.00000
%EndBlock PAO.Basis
```

*DZP*

```
%Block PAO.Basis
B      3         0.78484
  n=2     0     2     E      63.63953        5.37875
        6.10655        4.32596
        1.00000        1.00000
  n=2     1     2     E      70.56975        6.04344
        7.00887        5.13080
        1.00000        1.00000
  n=3     2     1     E     178.33839        0.36229
        5.47450
        1.00000
N      3        -0.01080
  n=2     0     2     E      89.26055        6.14782
        6.64924        4.76284
        1.00000        1.00000
  n=2     1     2     E      50.41573        3.95952
        6.22357        4.50898
        1.00000        1.00000
  n=3     2     1     E     117.80742        5.20126
        6.11679
        1.00000
%EndBlock PAO.Basis
```

*DZPF*

```
%Block PAO.Basis
B     4          0.65690
 n=2    0    2    E     36.99719        5.48219
     6.10787       4.31695
     1.00000       1.00000
 n=2    1    2    E      8.15973        3.80500
     6.00066       4.23675
     1.00000       1.00000
 n=3    2    1    E    165.32330        0.15783
     5.22533
     1.00000
 n=4    3    1    E      9.84678        3.95492
     6.03039
     1.00000
N     4          0.11571
 n=2    0    2    E     12.09088        5.41893
     6.00097       4.29407
     1.00000       1.00000
 n=2    1    2    E     62.94325        6.33211
     6.93370       4.89041
     1.00000       1.00000
 n=3    2    1    E     96.73771        5.41800
     5.91845
     1.00000
 n=4    3    1    E     80.94858        4.60177
     5.98908
     1.00000
%EndBlock PAO.Basis
```

*TZP*

```
%Block PAO.Basis
B     3          0.95935
 n=2    0    3    E     24.77915        5.84930
     6.64607       4.70140       2.80952
     1.00000       1.00000       1.00000
 n=2    1    3    E      2.80291        4.30124
     6.45810       4.58321       2.65142
     1.00000       1.00000       1.00000
 n=3    2    1    E     37.56157        3.08772
     6.02009
     1.00000
N     3         -0.15002
 n=2    0    3    E     39.51765        5.56899
     6.45792       4.57803       2.68043
     1.00000       1.00000       1.00000
 n=2    1    3    E    139.37566        6.35024
     7.01448       5.06017       2.93135
     1.00000       1.00000       1.00000
 n=3    2    1    E     53.49722        3.01864
     6.08186
     1.00000
%EndBlock PAO.Basis
```

*TZPF*

```
%Block PAO.Basis
B       4           0.31564
  n=2     0     3     E       78.71323         4.51053
        6.35162        4.46434        2.78530
        1.00000        1.00000        1.00000
  n=2     1     3     E      105.85276         5.21075
        6.08135        4.32741        2.56344
        1.00000        1.00000        1.00000
  n=3     2     1     E      196.88539         0.02236
        5.79992
        1.00000
  n=4     3     1     E      204.83656         5.53969
        6.09516
        1.00000
N       4          -0.36719
  n=2     0     3     E       75.15812         4.69696
        6.30460        4.46314        2.61741
        1.00000        1.00000        1.00000
  n=2     1     3     E       87.54187         6.22568
        6.75624        4.77736        2.88117
        1.00000        1.00000        1.00000
  n=3     2     1     E      139.66255         0.00057
        5.47231
        1.00000
  n=4     3     1     E       17.91544         1.66331
        5.57721
        1.00000
%EndBlock PAO.Basis
```

*QZP*

```
%Block PAO.Basis
B       3           0.62707
  n=2     0     4     E       47.55703         3.74326
        6.00236        4.24254        2.52313        1.56234
        1.00000        1.00000        1.00000        1.00000
  n=2     1     4     E       53.66759         5.29311
        6.00032        4.30206        2.80946        1.82923
        1.00000        1.00000        1.00000        1.00000
  n=3     2     1     E      168.97419         0.27700
        5.20746
        1.00000
N       3          -0.29190
  n=2     0     4     E      148.33867         5.46181
        6.00406        4.28090        2.61584        1.50330
        1.00000        1.00000        1.00000        1.00000
  n=2     1     4     E       71.67199         6.27279
        6.94200        5.01383        2.98286        1.93924
        1.00000        1.00000        1.00000        1.00000
  n=3     2     1     E      239.30730         0.51431
        4.69691
        1.00000
%EndBlock PAO.Basis
```

*QZPF*

```
%Block PAO.Basis
B    4      0.95282
 n=2   0   4   E    90.45980     4.02063
     6.00261     4.35769     3.06913     1.50842
     1.00000     1.00000     1.00000     1.00000
 n=2   1   4   E    17.71235     5.10128
     6.19558     4.12904     2.64408     1.90308
     1.00000     1.00000     1.00000     1.00000
 n=3   2   1   E   151.22707     0.09582
     5.14522
     1.00000
 n=4   3   1   E   241.64891     3.72896
     4.69182
     1.00000
N    4     -0.39742
 n=2   0   4   E   242.80866     5.52356
     6.03693     4.22935     2.53630     1.99224
     1.00000     1.00000     1.00000     1.00000
 n=2   1   4   E   117.50929     6.17355
     6.68422     4.77836     3.07390     2.03596
     1.00000     1.00000     1.00000     1.00000
 n=3   2   1   E   224.22459     0.09455
     5.69080
     1.00000
 n=4   3   1   E   248.76852     0.73985
     4.75821
     1.00000
%EndBlock PAO.Basis
```

**NATIVE BASIS SETS**

**Graphene**

*SZP*

```
%block PAO.Basis
C                   3
 n=2   0   1
   5.519
   1.000
 n=2   1   1
   7.086
   1.000
 n=3   2   1
   7.086
   1.000
%endblock PAO.Basis
```

*SZPF*

```
%block PAO.Basis
C                   4
 n=2   0   1
```

```
    5.519
    1.000
  n=2    1    1
    7.086
    1.000
  n=3    2    1
    7.086
    1.000
  n=4    3    1
    7.086
    1.000
%endblock PAO.Basis
```

*DZP*

```
%block PAO.Basis
C                          3
  n=2    0    2
    5.519        3.475
    1.000        1.000
  n=2    1    2
    7.086        3.793
    1.000        1.000
  n=3    2    1
    7.086
    1.000
%endblock PAO.Basis
```

*DZPF*

```
%block PAO.Basis
C                          4
  n=2    0    2
    5.519        3.519
    1.000        1.000
  n=2    1    2
    7.086        3.793
    1.000        1.000
  n=3    2    1
    7.086
    1.000
  n=4    3    1
    7.086
    1.000
%endblock PAO.Basis
```

*TZP*

```
%block PAO.Basis
C                          3
  n=2    0    3
    5.519        3.475        3.987
    1.000        1.000        1.000
  n=2    1    3
    7.086        3.793        4.518
    1.000        1.000        1.000
```

```
  n=3    2    1
    7.086
    1.000
%endblock PAO.Basis
```

*TZPF*

```
%block PAO.Basis
C                          4
  n=2    0    3
    5.519       3.519       3.987
    1.000       1.000       1.000
  n=2    1    3
    7.086       3.793       4.518
    1.000       1.000       1.000
  n=3    2    1
    7.086
    1.000
  n=4    3    1
    7.086
    1.000
%endblock PAO.Basis
```

*QZP*

```
%block PAO.Basis
C                          3
  n=2    0    4
    5.519       3.475       3.987       4.462
    1.000       1.000       1.000       1.000
  n=2    1    4
    7.086       3.793       4.518       5.184
    1.000       1.000       1.000       1.000
  n=3    2    1
    7.086
    1.000
%endblock PAO.Basis
```

*QZPF*

```
%block PAO.Basis
C                          3
  n=2    0    4
    5.519       3.475       3.987       4.462
    1.000       1.000       1.000       1.000
  n=2    1    4
    7.086       3.793       4.518       5.184
    1.000       1.000       1.000       1.000
  n=3    2    1    P  1
    7.086
    1.000
%endblock PAO.Basis
```

**hBN**

*SZP*

```
%block PAO.Basis
B                    3
 n=2   0   1
   6.459
   1.000
 n=2   1   1
   8.294
   1.000
 n=3   2   1
   8.294
   1.000
N                    3
 n=2   0   1
   4.850
   1.000
 n=2   1   1
   6.228
   1.000
 n=3   2   1
   6.228
   1.000
%endblock PAO.Basis
```

*SZPF*

```
%block PAO.Basis
B                    4
 n=2   0   1
   6.459
   1.000
 n=2   1   1
   8.294
   1.000
 n=3   2   1
   8.294
   1.000
 n=4   3   1
   8.294
   1.000
N                    4
 n=2   0   1
   4.850
   1.000
 n=2   1   1
   6.228
   1.000
 n=3   2   1
   6.228
   1.000
 n=4   3   1
   6.228
   1.000
%endblock PAO.Basis
```

*DZP*

```
%block PAO.Basis
B                     3
 n=2   0   2
   6.459      4.276
   1.000      1.000
 n=2   1   2
   8.294      4.785
   1.000      1.000
 n=3   2   1
   8.294
   1.000
N                     3
 n=2   0   2
   4.850      2.942
   1.000      1.000
 n=2   1   2
   6.228      3.131
   1.000      1.000
 n=3   2   1
   6.228
   1.000
%endblock PAO.Basis
```

*DZPF*

```
%block PAO.Basis
B                     4
 n=2   0   2
   6.459      4.329
   1.000      1.000
 n=2   1   2
   8.294      4.785
   1.000      1.000
 n=3   2   1
   8.294
   1.000
 n=4   3   1
   8.294
   1.000
N                     4
 n=2   0   2
   4.850      2.942
   1.000      1.000
 n=2   1   2
   6.228      3.171
   1.000      1.000
 n=3   2   1
   6.228
   1.000
 n=4   3   1
   6.228
   1.000
%endblock PAO.Basis
```

*TZP*

```
%block PAO.Basis
B                       3
 n=2    0    3
   6.459        4.276        4.906
   1.000        1.000        1.000
 n=2    1    3
   8.294        4.785        5.629
   1.000        1.000        1.000
 n=3    2    1
   8.294
   1.000
N                       3
 n=2    0    3
   4.850        2.942        3.375
   1.000        1.000        1.000
 n=2    1    3
   6.228        3.131        3.777
   1.000        1.000        1.000
 n=3    2    1
   6.228
   1.000
%endblock PAO.Basis
```

*TZPF*

```
%block PAO.Basis
B                       4
 n=2    0    3
   6.459        4.329        4.906
   1.000        1.000        1.000
 n=2    1    3
   8.294        4.785        5.700
   1.000        1.000        1.000
 n=3    2    1
   8.294
   1.000
 n=4    3    1
   8.294
   1.000
N                       4
 n=2    0    3
   4.850        2.942        3.418
   1.000        1.000        1.000
 n=2    1    3
   6.228        3.171        3.777
   1.000        1.000        1.000
 n=3    2    1
   6.228
   1.000
 n=4    3    1
   6.228
   1.000
%endblock PAO.Basis
```

*QZP*

```
%block PAO.Basis
B                          3
  n=2    0    4
    4.785        4.118        4.551        4.667
    1.000        1.000        1.000        1.000
  n=2    1    4
    5.700        4.223        4.845        5.355
    1.000        1.000        1.000        1.000
  n=3    2    1
    8.294
    1.000
N                          3
  n=2    0    4
    3.684        2.869        3.251        3.504
    1.000        1.000        1.000        1.000
  n=2    1    4
    4.280        2.905        3.375        3.777
    1.000        1.000        1.000        1.000
  n=3    2    1
    6.228
    1.000
%endblock PAO.Basis
```

*QZPF*

```
%block PAO.Basis
B                          4
  n=2    0    4
    4.785        4.118        4.551        4.667
    1.000        1.000        1.000        1.000
  n=2    1    4
    5.700        4.223        4.906        5.422
    1.000        1.000        1.000        1.000
  n=3    2    1
    8.294
    1.000
  n=4    3    1
    8.294
    1.000
N                          4
  n=2    0    4
    3.684        2.869        3.251        3.504
    1.000        1.000        1.000        1.000
  n=2    1    4
    4.280        2.942        3.418        3.777
    1.000        1.000        1.000        1.000
  n=3    2    1
    6.228
    1.000
  n=4    3    1
    6.228
    1.000
%endblock PAO.Basis
```
